# Supplementary material for: Selective, Interpretable, and Motion Consistent Privacy Attribute Obfuscation for Action Recognition
Source: arXiv:2403.12710 source file (2024-03-19)
Supplement: Supplementary file 1 [file X_suppl.tex]

\clearpage
\setcounter{page}{1}
\maketitlesupplementary

%\todo{FILIP: Since this document will be submitted separately from the main: (1) I've reset the section heading count; (2) I've reset the figure counters and (3) also need to make sure that citations to the main paper, \eg equation numbers and references, work properly. For example, it likely will be necessary to enter by hand the equation numbers that refer to the main paper and to include a separate biblio -- typically, that's been necessary in the past. }

\setcounter{section}{0}
\setcounter{figure}{0}
\setcounter{equation}{0}
\setcounter{table}{0}

\section{Supplemental video}
\noindent We present a method for obfuscation in \textit{videos} that relies on temporally consistent noise. It is therefore important to view the supplemental video: \texttt{\textbf{10410.mp4}} (\texttt{H.264, MPEG-4 AAC}). The video also contains an audio track with narration. It is approximately four minutes in length.
The examples mentioned in the main paper that reference the supplement (especially those that focus on the temporal aspect of the obfuscation) are found in the video as they cannot be demonstrated effectively in a pdf.

% \vspace{4em}
\section{Implementation details}

%\vspace{0.5em}\noindent\textbf{Motion consistent noise.}
\subsection{Motion consistent noise}
For the creation of motion consistent noise, we follow \cite{ilic2022appearance} that uses RAFT~\cite{RAFT} for optical flow estimation and nearest neighbor interpolation during warping.
We also highlight that using noise that is adjusted to the dataset mean, main submission \eqref{eq:afdinit}, is important, as other initializations reduce classification performance.

%\vspace{0.5em}\noindent\textbf{Matcher - queries, keys or values?}
\subsection{Matcher - queries, keys or values?}
For the template matcher, main submission Figure~\ref{fig:matching}, note that we use the \textit{keys} of the vision transformer. This choice follows related work, \eg~\cite{amir2021deep, oquab2023dinov2}; however, in our preliminary experiments we did not find large differences in using either \textit{values} or \textit{queries}, rather than \textit{keys}.

Figure \ref{fig:suppl_sim} provides additional examples of saliency maps, main submission~\eqref{eq:saliencyMap}, across different individuals. As in the main paper the results shown are produced by matching the keys of the templates with the source images.
Note how the features generalize very well across different appearances, again highlighting their ability to capture the semantics with high spatial fidelity.

%\vspace{0.5em}\noindent\textbf{Additional training details.} 
\subsection{Additional training details}
For data augmentation: Videos are randomly resized to introduce scale variation and center cropped to $224\times224$ pixels. Horizontal flip augmentations are used for SBU and KTH, but not in IPN as the direction of the motion determines the class for some gestures. Colour and temporal jitter are applied, and input sequences are padded with the last frame in case the sequence is not long enough to fit the required clip length of a network. For two-stream approaches, both streams use the same spatial crops as the source video.
All spatial augmentations also are applied to privacy networks.

Note that while the action and privacy recognition algorithms are trained on the original datasets used for evaluation \cite{ipn,sbu,kth}, they are not trained on our obfuscated videos. In comparison, alternative compared state-of-the-art approaches do train recognition algorithms on their processed videos \cite{ryoo2017privacy,pahmdb,bqn}.

% \section*{Dataset details}

% Foo.

\begin{figure}[!t]
	\centering
	\includegraphics[width=\linewidth]{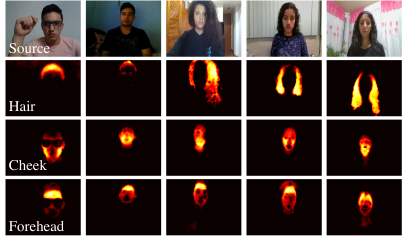}
	\vspace{-2em}
	\caption{Additional Saliency Maps Across Different Individuals Taken From the IPN Dataset.}
	\label{fig:suppl_sim}
\end{figure}
	
\begin{figure}[!t]
	\centering
	{
	\setlength{\tabcolsep}{1pt}
	\begin{tabularx}{\linewidth}{YYYYYY}
	\includegraphics[width=\linewidth]{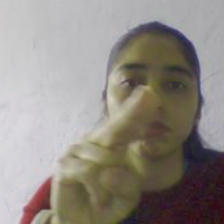}&%
	\includegraphics[width=\linewidth]{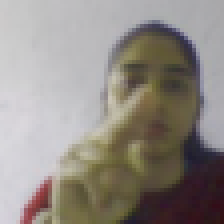}&%
	\includegraphics[width=\linewidth]{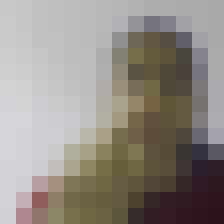}&%
	\includegraphics[width=\linewidth]{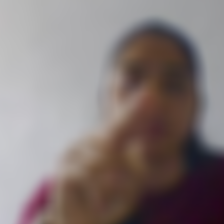}&%
	\includegraphics[width=\linewidth]{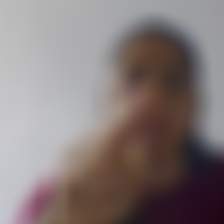}&%
	\includegraphics[width=\linewidth]{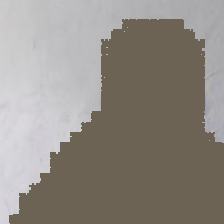}\\%
	\includegraphics[width=\linewidth]{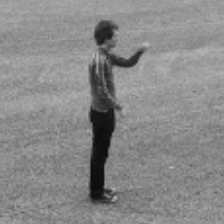}&%
	\includegraphics[width=\linewidth]{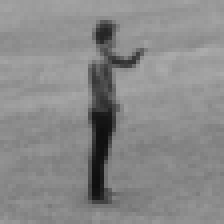}&%
	\includegraphics[width=\linewidth]{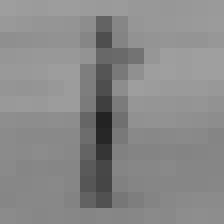}&%
	\includegraphics[width=\linewidth]{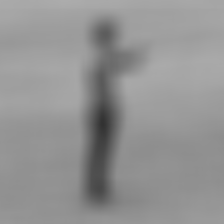}&%
	\includegraphics[width=\linewidth]{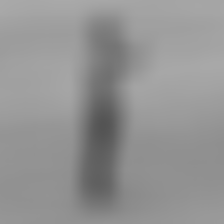}&%
	\includegraphics[width=\linewidth]{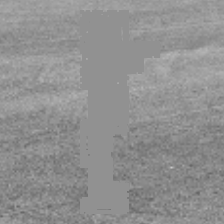}\\%
	\includegraphics[width=\linewidth]{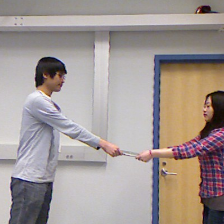}&%
	\includegraphics[width=\linewidth]{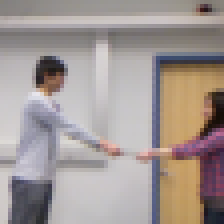}&%
	\includegraphics[width=\linewidth]{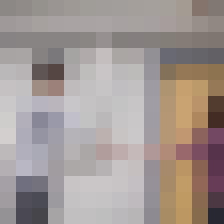}&%
	\includegraphics[width=\linewidth]{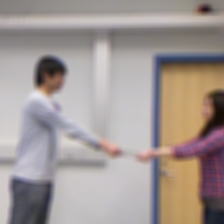}&%
	\includegraphics[width=\linewidth]{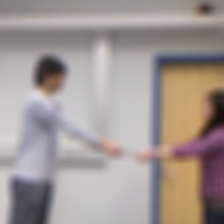}&%
	\includegraphics[width=\linewidth]{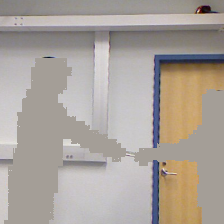}\\%
	Raw&%
        $\underset{4 \times 4}{\text{Pix}}$&
        $\underset{16 \times 16}{\text{Pix}}$&
        $\underset{\text{Weak}}{\text{Blur}}$&
        $\underset{\text{Strong}}{\text{Blur}}$&
	Mask\\%
	\end{tabularx}
	}
	\vspace{-1em}
	\caption{Qualitative Examples of  \textsc{Naive Baseline} Obfuscation Methods. These results augment those in main submission Figure \ref{fig:opticalflow}, which provided similar examples for state-of-the-art methods. Samples top-to-bottom are from IPN, KTH and SBU.}
 \label{fig:baselinequalitative}
\end{figure}

\begin{figure*}[!t]
	%COLORMAP WRT TO EACH DATASET
	\centering
	\begin{tabularx}{\linewidth}{YYY}%
		\includegraphics[width=1\linewidth]{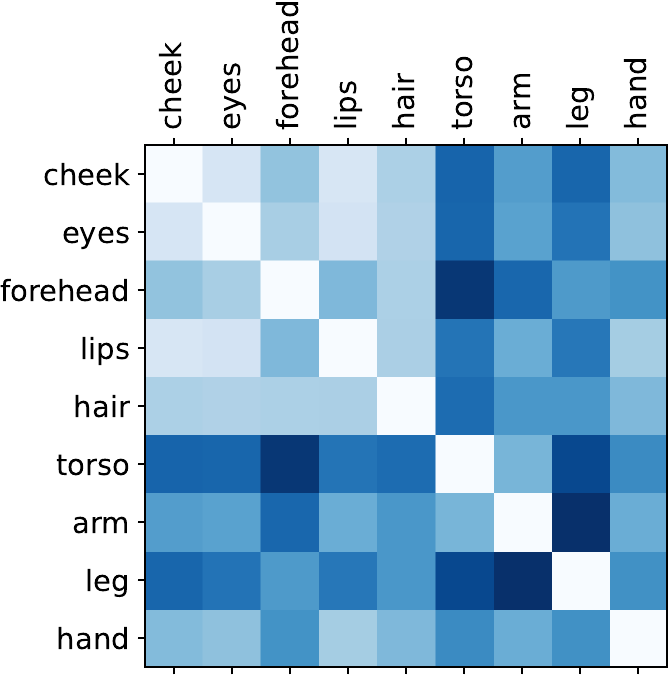} & 
		\includegraphics[width=1\linewidth]{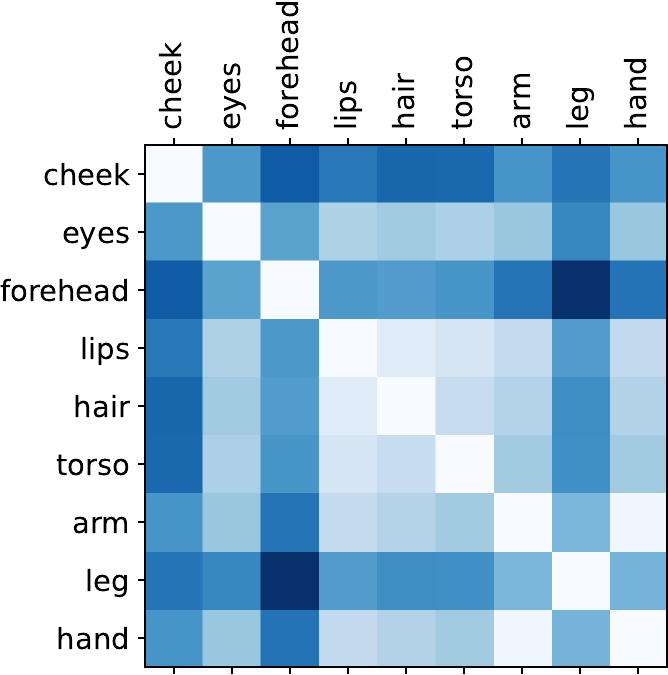} & 
		\includegraphics[width=1\linewidth]{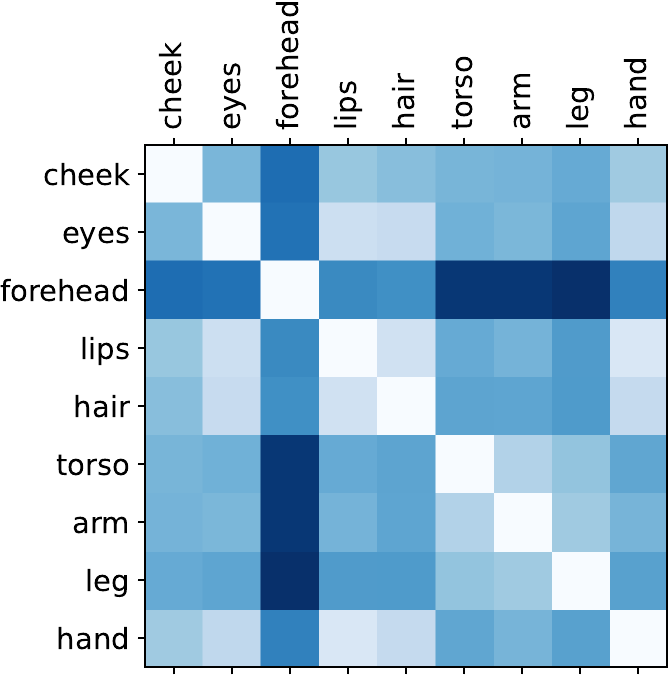}\\
		\qquad \quad IPN & \qquad \quad KTH & \qquad \quad SBU\\%
	\end{tabularx} %
	\vspace{-1em}
    \caption{Mean Average Error Between the Average Template Saliency for Each Dataset. Values plotted so that brighter values indicate that two templates are more similar to each other. The constructed matrices are diagonally symmetric by definition, \eqref{eq:templateSimilarity}.}
   \label{fig:mutual}
\end{figure*}

\section{Additional empirical evaluation}

\subsection{Naive baselines}
To get a better understanding of the naive baselines, we show samples from each of the three different datasets with all of the naive baseline obfuscation methods in Figure~\ref{fig:baselinequalitative}. As noted in the main submission, for the case of mask obfuscation the masking is performed by using the mean of the region covered by the mask.

%\vspace{0.5em}\noindent\textbf{Mask obfuscation.} 
In the main submission, we used the mean of the region in the original image covered by the mask to fill the region. As a variation, we also considered using black for the masked region. Use of the mean value, rather than black, improved the action recognition results on all three datasets  IPN \good{$+3.2$\% points}, KTH \good{$+1.3$\% points}, and SBU \good{$+2.4$\% points}; however, the differences on privacy attributes were small across all datasets: IPN \textcolor{red}{$+0.6$\% points}, KTH \good{$-0.3$\% points}, and SBU \good{$-0.2$\% points}. (We use \good{green} and \textcolor{red}{red} to indicate desired vs. undesired changes, respectively.)

% \begin{figure}[!h]
% 	COLORMAP NORMALIZED ACROSS DATASETS
% 	\centering
%        \includegraphics[width=0.8\linewidth]{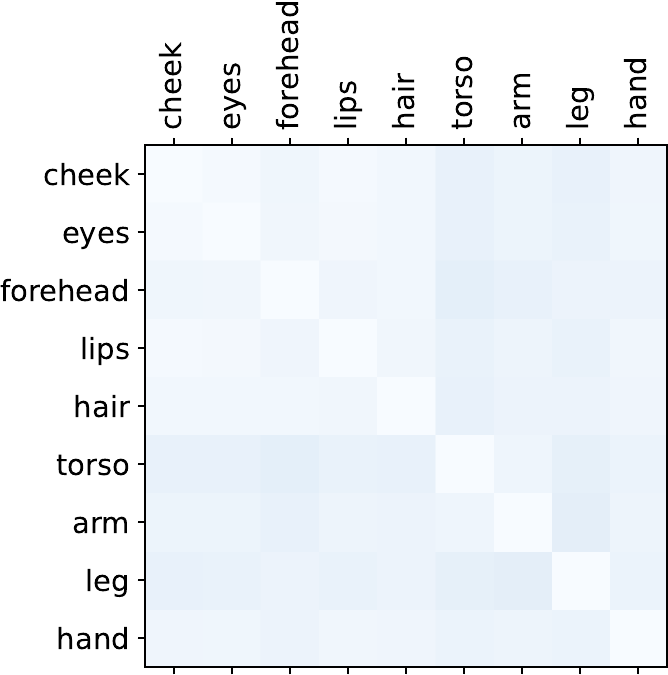}\\
% 	   \qquad \qquad IPN\\
%         \includegraphics[width=0.8\linewidth]{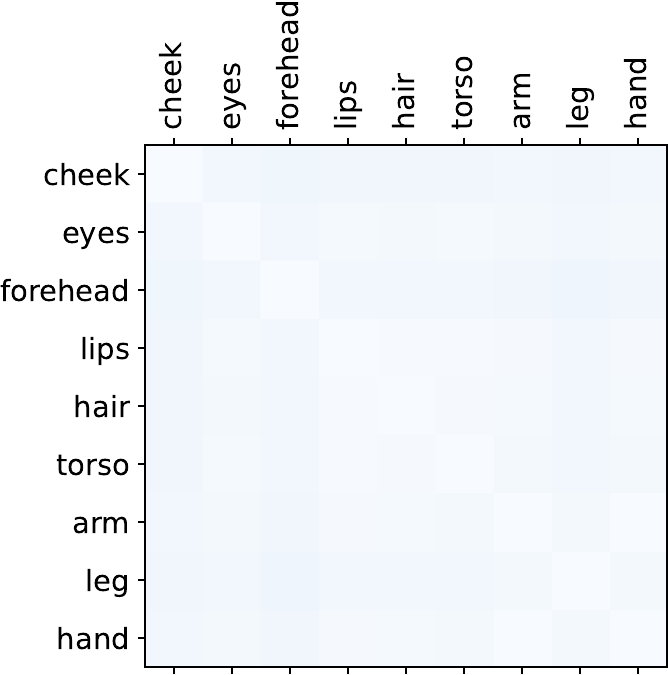}\\
% 		\qquad \qquad KTH\\
% 		\includegraphics[width=0.8\linewidth]{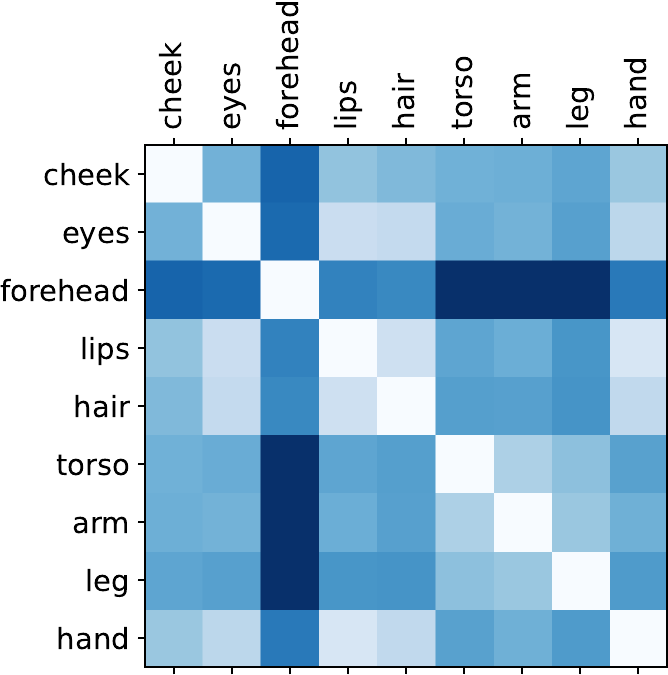}\\
% 		\qquad \qquad SBU
%     \caption{Mean Average Error Between the Average Template Saliency for Each Dataset. Values plotted so that lighter values indicate that two templates are more similar to each other. The constructed matrices are diagonally symmetric by definition, \eqref{eq:templateSimilarity}.}
%    \label{fig:mutual_normalized}
% \end{figure}

\subsection{Ablation over $f_\lambda$}
In the main submission, we introduced $f_\lambda$, \eqref{eq:metric}, as a way to rank multiple obfuscation methods by combining the two metrics of concern, \ie action recognition and privacy preservation, into a single value. 
Main submission Figure~\ref{fig:averagemetricsplot} showed the ranking and performance of obfuscation methods based on the importance weighting between action recognition and privacy preservation. In that figure, we averaged the results across our different datasets, here we provide the full ablation plots per dataset in Figure \ref{fig:metricsplot}.
The individual dataset ablations show that our method performs best across all datasets, and not just on average as shown in the main submission.

\subsection{Overlap of individual saliency maps}
As discussed in the main submission, the selection of the privacy templates is dependent on the task and the videos in the dataset, \eg there is no need to obscure lower body features for cases where only the upper body is visible in the video (IPN) and seeking to obscure detailed facial features when they are not distinguishable due to viewing at a great distance (KTH) also is not merited.
Here, we quantify the similarity of selected templates. One way to do this would be to measure the Euclidean distance of the descriptors, but that does not reveal how the obfuscation actually appears in a given dataset. Therefore, to measure the similarity between the templates on a dataset level, we compare the saliency maps directly.

In particular, we compute the average saliency map for each template, $\tau_k$ in the template library, $\mathsf{T}$, per dataset, according to
%$\bar{S}_{\tau_k}$, where  $\tau_k$ is the template under consideration from the entire library, $\mathsf{T}$, \ie
\begin{equation}
	\bar{S}_{\tau_k}(\mathbf{p}) = \frac{1}{n}\sum_{i=1}^n S_i(\mathbf{p}) \qquad  \forall \tau_k \in \sf{T},
\end{equation}
where $\mathbf{p} = (x,y)$ indexes pixels, $i$ indexes saliency maps and $n$ is the number of images in the dataset. (Main submission \eqref{eq:saliencyMap} provides the definition of individual salience maps.)
These averages allow us to compute the mean absolute error between the salience of all template pairs, $\tau_i$ and $\tau_j$,  as

\begin{equation}\label{eq:templateSimilarity}
			 v_{i,j} = \sum_{\mathbf{p}} | \bar{S}_{\tau_i}(\mathbf{p}) - \bar{S}_{\tau_j}(\mathbf{p})|,\end{equation}
with $\mathbf{p}$ ranging over all pixels in the average saliency maps. 

Figure~\ref{fig:mutual} shows the values, $v_{i,j}$, plotted so that greater similarity is visualized as brighter intensity.

From these plots, a number of observations can be made. First, it is seen that for all datasets the largest values appear along the diagonal, as templates should be most similar to themselves, and our similarity plots capture that property. Second, there is a tendency for templates with close spatial proximity to yield more similar saliency maps compared to those that are more distant. For example, templates for fine facial features, ``eyes, lips, cheek'', tend to yield saliency maps more similar to each other than to more distant body parts, ``torso, arm, hand'', and vice versa. Third, there is an interaction between spatial support and template similarity: If there is very little spatial support for a template, \eg fine facial features on KTH, then it results in relatively low similarity scores, as there is too little data to capture similarities.  

\begin{figure}[!t]
	\centering
	\resizebox{!}{3.5cm}{%
            \begin{tikzpicture}
		\begin{axis}[
			title={IPN},
			xlabel={$\leftarrow$ Action $ \qquad \lambda \qquad $ Privacy $\rightarrow$},
			ylabel={Bad$ \leftarrow  f_\lambda  \rightarrow$ Good},
			xmin=0, xmax=1.0,
			ymin=0, ymax=1.0,
			xtick={0.20,0.40,0.60,0.80,1.0},
			ytick={0.0,0.20,0.40,0.60,0.80,1.0,1.2},
			legend pos=outer north east,
			ymajorgrids=true,
			xmajorgrids=true,
			grid style=dashed,
			colormap name=bright, % activate the defined colormap
			cycle list={[of colormap]},
			every axis plot/.append style={mark=square*,ultra thick},
			legend cell align={left},
			width=7cm,
			height=4.35cm,
			yticklabel style={/pgf/number format/.cd,
            fixed,
            fixed zerofill,
            precision=1,
			/tikz/.cd},
			xticklabel style={/pgf/number format/.cd,
            fixed,
            fixed zerofill,
            precision=1,
			/tikz/.cd},
			]
		]
		\addplot+[]
		coordinates {
		(0.00, 0.85)(1.00, 0.41)};
		\addlegendentry{BDQ \cite{bqn}}
		
		\addplot+[]
		coordinates {
		(0.00, 0.81)(1.00, 0.35)};
		\addlegendentry{ALF \cite{pahmdb}}
		
		\addplot+[]
		coordinates {
		(0.00, 0.86)(1.00, 0.36)};
		\addlegendentry{ELR\cite{ryoo2018extremelowres} s=16}
		
		\addplot+[]
		coordinates {
		(0.00, 0.77)(1.00, 0.37)};
		\addlegendentry{ELR\cite{ryoo2018extremelowres} s=32}
		
		\addplot+[style={mark=square*,ultra thick}]
		coordinates {
		(0.00, 0.87)(1.00, 0.45)};
		\addlegendentry{Ours \textdagger}
		
		\addplot+[style={mark=square*,ultra thick}]
		coordinates {
		(0.00, 0.84)(1.00, 0.46)};
		\addlegendentry{Ours}
		\end{axis}
	\end{tikzpicture}
	}\\%
	\resizebox{!}{3.5cm}{%
            \begin{tikzpicture}
		\begin{axis}[
			title={KTH},
			xlabel={$\leftarrow$ Action $ \qquad \lambda \qquad $ Privacy $\rightarrow$},
			ylabel={Bad$ \leftarrow  f_\lambda  \rightarrow$ Good},
			xmin=0, xmax=1.0,
			ymin=0, ymax=1.0,
			xtick={0.20,0.40,0.60,0.80,1.0},
			ytick={0.0,0.20,0.40,0.60,0.80,1.0,1.2},
			legend pos=outer north east,
			ymajorgrids=true,
			xmajorgrids=true,
			grid style=dashed,
			colormap name=bright, % activate the defined colormap
			cycle list={[of colormap]},
			every axis plot/.append style={mark=square*,ultra thick},
			legend cell align={left},
			width=7cm,
			height=4.35cm,
			yticklabel style={/pgf/number format/.cd,
            fixed,
            fixed zerofill,
            precision=1,
			/tikz/.cd},
			xticklabel style={/pgf/number format/.cd,
            fixed,
            fixed zerofill,
            precision=1,
			/tikz/.cd},
			]
		]
		\addplot+[]
coordinates {
(0.00, 0.85)(1.00, 0.93)};
\addlegendentry{BDQ \cite{bqn}}

\addplot+[]
coordinates {
(0.00, 0.81)(1.00, 0.81)};
\addlegendentry{ALF \cite{pahmdb}}

\addplot+[]
coordinates {
(0.00, 0.86)(1.00, 0.11)};
\addlegendentry{ELR\cite{ryoo2018extremelowres} s=16}

\addplot+[]
coordinates {
(0.00, 0.77)(1.00, 0.17)};
\addlegendentry{ELR\cite{ryoo2018extremelowres} s=32}

\addplot+[style={mark=square*,ultra thick}]
coordinates {
(0.00, 0.87)(1.00, 0.95)};
\addlegendentry{Ours \textdagger}

\addplot+[style={mark=square*,ultra thick}]
coordinates {
(0.00, 0.84)(1.00, 0.96)};
\addlegendentry{Ours}
		\end{axis}
	\end{tikzpicture}
	}\\%
	\resizebox{!}{3.5cm}{%
		\begin{tikzpicture}
		\begin{axis}[
			title={SBU},
			xlabel={$\leftarrow$ Action $ \qquad \lambda \qquad $ Privacy $\rightarrow$},
			ylabel={Bad$ \leftarrow  f_\lambda  \rightarrow$ Good},
			xmin=0, xmax=1.0,
			ymin=0, ymax=1.0,
			xtick={0.20,0.40,0.60,0.80,1.0},
			ytick={0.0,0.20,0.40,0.60,0.80,1.0,1.2},
			legend pos=outer north east,
			ymajorgrids=true,
			xmajorgrids=true,
			grid style=dashed,
			colormap name=bright, % activate the defined colormap
			cycle list={[of colormap]},
			every axis plot/.append style={mark=square*,ultra thick},
			legend cell align={left},
			width=7cm,
			height=4.35cm,
			yticklabel style={/pgf/number format/.cd,
            fixed,
            fixed zerofill,
            precision=1,
			/tikz/.cd},
			xticklabel style={/pgf/number format/.cd,
            fixed,
            fixed zerofill,
            precision=1,
			/tikz/.cd},
			]
		]
		\addplot+[]
		coordinates {
		(0.00, 0.85)(1.00, 0.66)};
		\addlegendentry{BDQ \cite{bqn}}
		
		\addplot+[]
		coordinates {
		(0.00, 0.81)(1.00, 0.52)};
		\addlegendentry{ALF \cite{pahmdb}}
		
		\addplot+[]
		coordinates {
		(0.00, 0.86)(1.00, 0.17)};
		\addlegendentry{ELR\cite{ryoo2018extremelowres} s=16}
		
		\addplot+[]
		coordinates {
		(0.00, 0.77)(1.00, 0.35)};
		\addlegendentry{ELR\cite{ryoo2018extremelowres} s=32}
		
		\addplot+[style={mark=square*,ultra thick}]
		coordinates {
		(0.00, 0.87)(1.00, 0.88)};
		\addlegendentry{Ours \textdagger}
		
		\addplot+[style={mark=square*,ultra thick}]
		coordinates {
		(0.00, 0.84)(1.00, 0.87)};
		\addlegendentry{Ours}
		
		\end{axis}
	\end{tikzpicture}
	}%
	\caption{Per-Dataset Results of $\lambda$ Variation. These results augment those of main submission,  Figure~\ref{fig:averagemetricsplot} where results were averaged across datasets.}
	\label{fig:metricsplot}
\end{figure}

\begin{table}[!ht]
	\centering
	\footnotesize{\textsc{Action Recognition on \textbf{Our} obfuscation}}\vspace{0.5em}
		\begin{tabularx}{\linewidth}{lYYYY} % Updated to add 3 more columns
			\toprule
			\textbf{Network} & $f \times r$  & IPN & KTH & SBU\\
			\midrule
			\rc C2D \cite{wang2018non}& $ 8 \times 8 $ 					& 74.56 & 82.66 & 87.83 \\
			CSN \cite{tran2019video}& $ 32 \times 2 $ 					& 89.21 & 87.00 & 89.91 \\
			\rc E2S X3D L \cite{ilic2022appearance}& $ 16 \times 5 $ 	& 93.33 & 94.33 & 91.11 \\
			E2S X3D M \cite{ilic2022appearance}& $ 16 \times 5 $ 		& 89.01 & 92.33 & 88.76 \\
			\rc E2S X3D S \cite{ilic2022appearance}& $ 13 \times 6 $ 	& 85.16 & 90.33 & 84.10 \\
			I3D \cite{carreira2017quo} & $ 8 \times 8 $ 				& 85.25 & 89.87 & 84.04 \\
			\rc MVIT\cite{fan2021multiscale} & $ 16 \times 4 $ 			& 88.91 & 85.34 & 91.55 \\
			R2+1D \cite{tran2018closer} & $ 16 \times 4 $ 				& 88.78 & 87.33 & 82.09 \\
			\rc Slow \cite{feichtenhofer2019slowfast}& $ 8 \times 8 $ 	& 79.00 & 89.00 & 88.64 \\
			SlowFast \cite{feichtenhofer2019slowfast}& $ 32 \times 2 $ 	& 88.06 & 87.54 & 89.70 \\
			\rc X3D L \cite{feichtenhofer2020x3d}& $ 16 \times 5 $ 		& 93.11 & 91.00 & 93.66 \\
			X3D M \cite{feichtenhofer2020x3d}& $ 16 \times 5 $ 			& 90.19 & 88.30 & 83.38 \\
			\rc X3D S \cite{feichtenhofer2020x3d}& $ 13 \times 6 $ 		& 87.93 & 87.60 & 72.77 \\
			\midrule
			Average&  & 87.11 & 88.67 & 86.74 \\
			\bottomrule
		\end{tabularx}\\
		% \caption{Top-1 Accuracies of all Action Recognition Models; The average is reported as our "Action Recognition Accuracy"}
		% \label{tab:acion_detail}
		\vspace{1.2em}\footnotesize{\textsc{Privacy Preservation on \textbf{Our} obfuscation}}\vspace{0.5em}
		\begin{tabularx}{\linewidth}{lYYYY} % Updated to add 3 more columns
			\toprule
			\textbf{Network} & IPN & KTH& SBU\\
			\midrule
			\rc ResNet$_{18}$ \cite{he2016deep}  		& 49.59 & \phantom{0}4.29 & 11.78 \\
			ResNet$_{50}$ \cite{he2016deep}  			& 51.27 & \phantom{0}4.31 & 11.70 \\
			\rc ResNet$_{101}$ \cite{he2016deep} 		& 52.10 & \phantom{0}4.93 & 12.39\\
			ViT$_{b/16}$\cite{dosovitskiy2020image} 	& 52.98 & \phantom{0}6.56 & 14.98 \\
			\rc ViT$_{b/32}$\cite{dosovitskiy2020image} & 53.65 & \phantom{0}7.31 & 15.09 \\
			\midrule
			Average & 51.93 & 5.46 & 13.19\\
			\bottomrule
		\end{tabularx}
            \vspace{-0.5em}
		\caption{Top-1 Accuracy for all Privacy and Action models based on \textbf{Our} obfuscation method.}
		\label{tab:results_detail_ours}
\end{table}	

\subsection{Per model selective obfuscation}

In main submission Table~\ref{tab:results_detail}, we presented Top-1 accuracy for all privacy and action recognition models evaluated on
the original unmodified (source) videos, i.e. without our selective privacy obfuscation. In presenting privacy and action results with our obfuscation, we only presented results averaged across all models (or using just I3D when comparing to alternative state-of-the-art privacy preserving methods); see main submission Table~\ref{tab:results}. Here, we present per-model action and privacy results in Table~\ref{tab:results_detail_ours}. We see that our obfuscation always drastically impacts privacy, while having relatively less impact on action recognition, which is consistent with the on average results.
